# Supplementary material for: Finite-sample analysis of M-estimators using self-concordance
Source: arXiv:1810.06838 source file (2020-11-30)
Supplement: Supplementary file 1 [file robust-least-squares-appendix.tex]

\subsection{Basic deviation bounds}
\label{app:prob-tools}

\paragraph{Subgaussian distributions.}
The subgaussian norm of a random variable~$\xi \in \R$ is defined as
\[
\| \xi \|_{\psi_2} := \min \left\{c > 0 : \;\; \E \left[e^{\xi^2/c^2}\right] \le 2 \right\}.
\]
We call $\xi$ subgaussian if its subgaussian norm is finite (the notation $\psi_2$ corresponds to the fact that subgaussian random variables are those having a finite $2$-Orlicz norm as defined below). 
It is known~\cite{vershynin2010introduction} that there exists an absolute constant $c$ such that the following properties are equivalent:
\begin{itemize}
\item Subgaussian norm of $\xi$ is $\sigma$.
\item Tails:
\[
\Prob\left[|\xi| > t\right] \le \exp\left(1-\frac{ct^2}{\sigma^2}\right) \quad  \forall t \ge 0.
\]
\item Moments:
\[
\left(\E|\xi|^{p}\right)^{1/p} \le c\sigma \sqrt{p} \quad \forall p \ge 1.
\]
\end{itemize}
Moreover, if $\E \xi = 0$, then these properties are also equivalent to 
\begin{itemize}
\item Moment-generating function:
\[
\E \exp(t\xi) \le \exp(c\sigma^2t^2).
\]
\end{itemize}

\paragraph{Orlicz norms.}
A convex, strictly increasing function $\psi: \R_+ \to \R_+$ such that $\psi(0) = 0$ is called a \textit{Young function}.
For any random variable $\xi \in \R$, we can define the \textit{Orlicz norm} (for a thorough introduction into Orlicz norms, see e.g. \cite{pollard1990empirical}, \cite{buldygin2000metric}):
%\footnote{This norm is actually defined on distributions rather than random variables, but we keep things simple here.}
\[
\| \xi \|_{\psi_\alpha} := \min \left\{ c > 0 : \E \left[ \psi\left(\frac{|\xi|}{c}\right) \right]\le 1 \right\}.
\]
Note that Orlicz norm is a semi-norm for random variables defined on a common probabilty space. The following fact about Orlicz norms:
\begin{fact}\label{th:orlicz-max}
Given $N$ random variables $\xi_1, .., \xi_N \in \R$ having a finite $\psi$-norm. Then, 
\[
\E \left[\max_{1 \le i \le N} |\xi_i| \right] \le \psi^{-1}(N) \max_{1 \le i \le n} \|\xi_i\|_{\psi}.
\]
\end{fact}
\begin{proof}
We give the proof for the case where $\psi$ is twice differentiable on $t > 0$ (the general case follows since convex functions are twice differentiable almost everywhere). In this case, since by convexity $\psi'' \ge 0$, it follows that $\psi'$ is non-decreasing by the Newton-Leibniz formula. Hence, $\psi(a+b) \ge \psi(a) + \psi(b)$ for any $a,b \in \R_+$. Indeed, assuming w.l.o.g. that $a \le b$,
\[
\psi(a) = \int_{0}^a \psi'(t)dt \le \psi'(a)a \le \psi'(b)a \le \int_{b}^{a+b} \psi'(t)dt = \psi(a+b) - \psi(b).
\]
Hence, denoting $K = \max_{1 \le i \le n} \|\xi_i\|_{\psi}$, by Jensen's inequality we get
\begin{equation*}
\begin{aligned}
\frac{\E \max_{1 \le i \le N} |\xi_i|}{K} 
\le \psi^{-1} \left[ \E \psi\left(\frac{\max_{1 \le i \le N} |\xi_i|}{K}\right) \right]  
\le \psi^{-1} \left[ \E \psi\left(\sum_{1 \le i \le N}\frac{|\xi_i|}{\|\xi_i\|_{\psi}}\right) \right] \le \psi^{-1}(N).
\end{aligned}
\end{equation*}
\end{proof}
Following \cite{pollard1990empirical}, we consider the Orlicz norms corresponding to the following family of Young functions indexed by $\alpha > 0$:
\begin{align}\label{eq:orlicz-alpha}
&\psi_\alpha(t) := \left\{
\begin{aligned}
&\exp(t^{\alpha})-1, &\alpha \ge 1,\\
&\mathds{1}\left\{t \le \tau_\alpha \right\}k_\alpha t + \mathds{1}\left\{t \ge \tau_\alpha\right\}\exp(t^{\alpha}), & 0 < \alpha < 1,
\end{aligned}
\right.\\
&\text{where} \;\;  k_\alpha:= (\alpha e)^{1/\alpha},\;\; \text{and}\;\; \tau_\alpha = \alpha^{-1/\alpha}.\notag
\end{align}
Note that $\alpha = 2$ gives the subgaussian case, and $\alpha = 1$ corresponds to subexponential tails. $\alpha < 1$ give tails heavier than exponential; note that the function $\exp(t^{\alpha})$ is not convex on $\R_+$ when $\alpha < 1$, so we convexify it by linear extrapolation near the origin). 
We need to formulate some properties of Young functions. 
\begin{fact}\label{th:orlicz-inverse}
For any $\alpha > 0$ and $N \ge e^{1/\alpha}$, one has
\[
\psi_\alpha^{-1}(N) \le [\log(N+1)]^{1/\alpha}.
\]
\end{fact}
\begin{fact}\label{th:orlicz-power}
If $\xi$ has a finite $\psi_{\alpha}$-norm $K$ for some $\alpha$. then for any $p \ge 0$, we have
\[
\||\xi|^{p}\|_{\psi_{\alpha/p}} \le C_{\alpha} K^p,
\] 
where the constant $C_{\alpha}$ depends only on $\alpha$. In particular, the $\alpha/2$-power of a random variable with a finite $\psi_\alpha$-norm is subgaussian\footnote{This fact is related to the classical theory of Box-Cox transform \cite{box-cox}.}.

\begin{proof}
The fact follows from the following bound, which is easy to check directly:
\begin{equation}\label{eq:orlicz-bracket}
\exp(t^\alpha) - c_\alpha \le \psi_\alpha(t) \le \exp(t^\alpha),
\end{equation}
where $c_\alpha$ is a positive constant depending only on $\alpha$. Then, we can take $C_\alpha = 1+c_\alpha$. Indeed,
\begin{align*}
\E \psi_{\alpha/p} \left( \frac{|\xi|^p}{(1 + c_\alpha)K^p} \right) 
&\le \frac{1}{1+c_\alpha} \E \psi_{\alpha/p} \left( \frac{|\xi|^p}{K^p} \right) \\
&\le \frac{1}{1+c_\alpha} \E \exp \left( \left[ \frac{|\xi|}{K} \right]^{\alpha} \right) \\
&\le \frac{1}{1 + c_\alpha} \left( \E \psi_{\alpha} \left( \frac{|\xi|}{K} \right) + c_\alpha \right) \le 1.
\end{align*}
Here, we used $\psi(C t) \ge C \psi(t)$ for any $C \ge 1$, see the proof of Fact~\ref{th:orlicz-max}, and then \eqref{eq:orlicz-bracket} twice.
\end{proof}
%In particular, $|\xi|^{\alpha/2}$ has subgaussian norm upper-bounded by $(K_\alpha)^{\alpha/2}$. 
\end{fact}
%Note that  is equivalent to   $\xi^{\alpha/2} := |\xi|^{\alpha/2}  \text{sign}(\xi)$ having subgaussian norm $K^{\alpha/2}$.
We define Orlicz norm of a random vector $X \in \R^d$ as the maximum norm of its one-dimensional marginals:
\[
\|X\|_{\psi_\alpha} := \sup_{x \in \S^{d-1}} \|\langle X, x \rangle\|_{\psi_\alpha}.
\]

\subsection{Estimation of covariance matrices}
\label{app:cov-mat}
Let $\Sigma$ be a positive-definite $d \times d$ matrix, and consider a random vector $x \in \R^d$ with $\E x = 0$ and covariance matrix $\Sigma = \E[x \otimes x]$ (note that $z = \Sigma^{-1/2} x$ is isotropic, that is, has zero mean and unit covariance matrix). We are given a sample $x_1, ..., x_n$ and would like to estimate $\Sigma$ from it. By the central limit theorem, a good candidate estimator of $\Sigma$ is the sample covariance matrix.
\[
\widehat \Sigma := \frac{1}{n} \sum_{i=1}^n x_i \otimes x_i.
\]
\paragraph{Subgaussian tails.}
The following proposition quantifies convergence of sample covariance matrix for finite samples in the subgaussian case.
\begin{proposition}{\cite[Theorem 5.39, Remark 5.40]{vershynin2010introduction}.}
Let $x_1, ..., x_n$ be independent copies of a random vector $x \in \R^d$ with $\E x = 0$, $\E[x \otimes x] = \Sigma$, and $\| x \|_{\psi_2} \le K$. Then, for every $t \ge 0$, the following inequality holds with probability at least $1-2\exp(-c_Kt^2)$:
\begin{equation*}
\|\widehat \Sigma - \Sigma\| \le \max(\varepsilon, \varepsilon^2), \quad \text{where} \quad \varepsilon = C_K \sqrt{\frac{d}{n}} + \frac{t}{\sqrt{n}},
\end{equation*}
and one can take $c_K = 1/K^4$, $C_K = K^2$.
\end{proposition}
We provide a convenient reformulation of this statement which follows through a straightforward calculation, by putting $\varepsilon \le \frac{1}{2}$ and inverting the bound.
\begin{proposition}\label{th:subg-cov-prob}
Suppose that $\Sigma$, $\widehat \Sigma$, and $K$ are as above. If, for $\delta \in (0,1]$,
\[
n \gtrsim K^4 (d + \log(1/\delta)),
\]
one has, with probability at least $1-\delta$,
\begin{equation}\label{eq:subg-cov-prob}
\|\widehat \Sigma - \Sigma \| \le 1/2.
\end{equation}
\end{proposition}
We can use the above statement to obtain the equivalence of the Mahalanobis distances. For that, define the standardized vector $z = \Sigma^{-1/2} x$ such that $\E [z \otimes z] = I$, and denote $\widehat I$ the corresponding sample covariance matrix. Note that $\widehat \Sigma = \Sigma^{1/2} \widehat I \Sigma^{1/2}$, and hence we have the following fact which immediately implies the theorem stated below.
\begin{fact}\label{fact:mahalanobis-equiv} 
Inequality 
\[
\| \widehat I - I \| \le 1/2,
\]
implies the equivalence of the norms defined by $\Sigma$ and $\widehat \Sigma$: for any $w \in \R^d$,
\[
\frac{1}{2} \|\Sigma^{1/2} w\|^2_{2} \le \|\widehat \Sigma^{1/2} w\|^2_{2} \le \frac{3}{2} \|\Sigma^{1/2} w\|^2_{2}.
\]
\end{fact}
\begin{theorem}\label{th:covariance-subgaussian} 
Suppose that $x \in \R^d$, $\Sigma$ and $\widehat \Sigma$ are as above. Assume that the standardized design $z = \Sigma^{-1/2}x$ satisfies 
\[
\|z\|_{\psi_2} \le K.
\] 
If, for $\delta \in (0,1]$,
\[
n \gtrsim K^4 (d + \log(1/\delta)),
\]
one has, for any $w \in \R^d$, 
\[
\frac{1}{2} \|\Sigma^{1/2} w\|^2_{2} \le \|\widehat \Sigma^{1/2} w\|^2_{2} \le \frac{3}{2} \|\Sigma^{1/2} w\|^2_{2}
\]
with probability at least $1-\delta$.
\end{theorem}
\begin{proof}
Apply Proposition~\ref{th:subg-cov-prob} to the standardized design, then use Fact~\ref{fact:mahalanobis-equiv}.
\end{proof}

\paragraph{Heavy tails.} We now address the heavy-tailed case, where we can provide statements in expectation (and as such, with a constant probability). We will use the following functional of a random vector $x \in \R^d$:
\[
M(x) := \E \max_{i \le n} \|x_i\|_2^2.
\] 
%We start with a basic estimate.
\begin{proposition}{\cite[Theorem 5.48]{vershynin2010introduction}.}
\label{th:covariance-heavy}
Let $x_1, ..., x_n$ be independent copies of a random vector $x \in \R^d$ with $\E x = 0$ and covariance matrix $\E[x \otimes x] = \Sigma$. Suppose in addition that $\|\Sigma\| \le 1$. Then, for some absolute constant $C$,
\[
\E \|\widehat \Sigma - \Sigma \| \le \max(\varepsilon, \varepsilon^2), \quad \text{where} \quad \varepsilon = C \sqrt{\frac{M(x) \log (d)}{n}}.
\]
\end{proposition}
\begin{corollary}\label{th:M-log-d}
Under the assumptions of the previous proposition, it suffices to take $n \gtrsim M \log(d)$
in order to guarantee that
\begin{equation}\label{eq:unit-cov-exp}
\E \|\widehat \Sigma - \Sigma\| \le 1/12.
\end{equation}
\end{corollary}
Recall that we are trying to approximate the Mahalanobis distance induced by $\Sigma$ via that induced by $\widehat \Sigma$. For that purpose, we would like to apply the above theorem to the isotropic case $\Sigma = I$ to approximate $I$ by $\widehat I$ and then proceed as in the case of subgaussian tails. Here we do not assume subgaussian tails; nonetheless, the quantity $M$ can be controlled if we assume that $z$ has a finite $\alpha$-Orlicz norm (essentially, it means that one-dimensional marginals of $z$ have a finite $\alpha$-th exponential moment); this includes the subgaussian assumption when $\alpha = 2$.

%Note that in the isotropic case, $M \ge \max_{i \le n} \E \|x_i\|_2^2 = d$, and hence, if we want to require that $\varepsilon < 1/2$, we must take $n \gg d$ anyway, hence $\log(n \wedge d) = \log(d)$ for that purpose, and we obtain the following corollary.
\begin{theorem}\label{th:covariance-orlicz}
Suppose that the standardized design $z = \Sigma^{-1/2}x$ has a finite Orlicz norm $\| z \|_{\psi_\alpha}$, where $\psi_\alpha$ is defined by~\eqref{eq:orlicz-alpha} for some $\alpha > 0$. 
\begin{enumerate}
\item As long as $n \ge e^{1/\alpha}$, we have
\begin{equation}\label{eq:orlicz-1}
M(z) \le C_\alpha \| z \|_{\psi_\alpha} [\ln(n+1)]^{1/\alpha}d,
\end{equation}
where $C_\alpha$ depends only on $\alpha$. 
\item Moreover, if 
\begin{equation}\label{eq:orlicz-2}
\frac{n}{(\log (2n))^{1/\alpha}} \gtrsim \max\left( C_\alpha \| z \|^2_{\psi_\alpha} d \log(d), \; \exp(1/\alpha) \right),
\end{equation}
then, with probability at least $5/6$, for any $w \in \R^d$ it holds
\begin{equation}\label{eq:orlicz-3}
\frac{1}{2} \|\Sigma^{1/2} w\|^2_{2} \le \|\widehat \Sigma^{1/2} w\|^2_{2} \le \frac{3}{2} \|\Sigma^{1/2} w\|^2_{2}.
\end{equation}
\end{enumerate}
\end{theorem}
\begin{proof}
Let $z_{(i)}$ denote the components of $z$ for $i \le d$. First we bound the Orlicz norm of $\|z\|_2^2$:
\[ 
\left\| [\|z\|_2^2]  \right\|_{\psi_{\alpha/2}} \le \sum_{i=1}^d \left\| z_{(i)}^2  \right\|_{\psi_{\alpha/2}} \le C_\alpha \sum_{i=1}^d \left\| z_{(i)} \right\|^2_{\psi_{\alpha}} \le dC_\alpha \| z \|^2_{\psi_\alpha},
\]
where $C_\alpha > 0$ depends only on $\alpha$; here we used that $\|\cdot\|_{\psi_\alpha}$ is a semi-norm (triangle inequality), then Fact~\ref{th:orlicz-power} for $p=2$, and, finally, the definition of $\psi_\alpha$-norm of a random vector. Using Fact~\ref{th:orlicz-max} together with Fact~\ref{th:orlicz-inverse}, we get~\eqref{eq:orlicz-1}. For the second part of the theorem, note that Theorem~\ref{th:covariance-heavy} and Corollary~\ref{th:M-log-d} applied to the case $\Sigma = I$ give that $\E\|\widehat I - I\| \le 1/12$. Whence by Markov's inequality, $\|\widehat I - I\| \le 1/2$ with probability at least $5/6$, and it remains to recall Fact~\ref{fact:mahalanobis-equiv}.
\end{proof}

\paragraph{Regularized covariance matrices.}
In the case of heavy tails, we would also like to encompass the more general situation of regularized covariance matrices, which will subsequently be used in ridge regression. \footnote{As far as we are aware, it is an open question to generalize the subgaussian-tails results from the previous paragraph to the case of regularized covariance, without invoking boundedness assumptions.}. First, we need to introduce some new objects. We are to study the Mahalanobis distance induced by $\Sigma_\lambda := \Sigma + \lambda I$ for some $\lambda \ge 0$. Define a random vector
\[
\zeta := \Sigma_\lambda^{-1/2} x = \Sigma_\lambda^{-1/2} \Sigma^{1/2} z,
\]
whose covariance matrix
\[
J_\lambda := \Sigma_\lambda^{-1/2} \Sigma \Sigma_\lambda^{-1/2} = \Sigma_\lambda^{-1} \Sigma
\]
has eigenvalues 
\[
\nu_j := \frac{\lambda_j}{\lambda_j + \lambda},
\] 
where $\lambda_j$ are eigenvalues of $\Sigma$ sorted in the non-increasing order.
Next, for $p \ge 1$ define the \textit{$\ell_p$-number of degrees of freedom} for ridge regression is defined as 
\[
\df_{p} := \Tr(J_\lambda^p),
\]
where $\df_2$ is called simply the number of degrees of freedom in the literature. Here we will only be interested in the largest quantity $\df_1$. Note that \[\df_1 \le d,\] and the gap between $\df_1 \le d$ is wide if only a few $\lambda_j$ are greater than $\lambda$.
%and the effective rank
%\[
%r_\lambda := \max \{j \le d : \lambda_j \ge \lambda\},
%\] 
%with the convention $r_\infty = 0$. It is straightforward to check the following facts:
%\begin{align}
%&d_\lambda \le d. \label{eq:df-d}\\
%&r_\lambda \le 2 d_\lambda. \label{eq:r-df}\\
%&1/2 \le q_j \le 1 \quad \text{for} \;\; j \le r_\lambda.\label{eq:q-id}.
%\end{align}

Our goal now is to obtain the equivalence of $\widehat \Sigma_\lambda = \widehat \Sigma + \lambda I$ and $\Sigma_\lambda$ for large enough sample size. In the case $\lambda = 0$ we needed, essentially, $n \gtrsim d \log d$, as stated by Theorem~\ref{th:covariance-orlicz}. The following generalization of Theorem~\ref{th:covariance-orlicz} shows that in the general case, $d$ is replaced with $\df_1$.
\begin{theorem}\label{th:covariance-orlicz-ridge}
Suppose that the standardized design $z = \Sigma^{-1/2}x$ has a finite Orlicz norm $\| z \|_{\psi_\alpha}$, where $\psi_\alpha$ is defined by~\eqref{eq:orlicz-alpha} for some $\alpha > 0$.
\begin{enumerate}
\item As long as $n \ge e^{1/\alpha}$, we have
\begin{equation}\label{eq:orlicz-ridge-1}
M(\zeta) \le C_\alpha \| z \|_{\psi_\alpha} [\ln(n+1)]^{1/\alpha}\df_1,
\end{equation}
where $C_\alpha$ depends only on $\alpha$. 
\item Moreover, if 
\begin{equation}\label{eq:orlicz-ridge-2}
\frac{n}{(\log (2n))^{1/\alpha}} \gtrsim \max\left( C_\alpha \| z \|^2_{\psi_\alpha} \df_1 \log(\df_1), \;\exp(1/\alpha)\right),
\end{equation}
then with probability at least $5/6$, for any $w \in \R^d$ it holds
\begin{equation}\label{eq:orlicz-ridge-3}
\frac{1}{2} \|\Sigma_\lambda^{1/2} w\|^2_{2} \le \|\widehat \Sigma_\lambda^{1/2} w\|^2_{2} \le \frac{3}{2} \|\Sigma_\lambda^{1/2} w\|^2_{2}.
\end{equation}
\end{enumerate}
\end{theorem}
\begin{proof}
%The proof of the theorem mimics that of Theorem~\ref{th:covariance-orlicz}. 
Denote $\zeta_{(i)}$ the components of $\zeta$ and $z_{(i)}$ those of $z$. To prove~\eqref{eq:orlicz-ridge-1}, we may assume w.l.o.g. that $\Sigma$ is diagonal, since both the $\ell_2$-norm and the $\psi_\alpha$-norm are rotation-invariant. Similarly to the proof of \eqref{eq:orlicz-1},
\[ 
\left\| [\|\zeta\|_2^2]  \right\|_{\psi_{\alpha/2}} \le \sum_{i=1}^d \left\| \zeta_{(i)}^2  \right\|_{\psi_{\alpha/2}} =  \sum_{i=1}^d \nu_i \left\| z_{(i)}^2  \right\|_{\psi_{\alpha/2}} \le C_\alpha \sum_{i=1}^d \nu_i \left\| z_{(i)}\right\|^2_{\psi_{\alpha}} \le C_\alpha \df_1 \| z \|^2_{\psi_\alpha},
\]
and~\eqref{eq:orlicz-ridge-1} follows as in Theorem~\ref{th:covariance-orlicz}. 
For the second part, first note that $\|J_\lambda\| = \nu_1 \le 1$, and hence Proposition~\ref{th:covariance-heavy} and Corollary~\ref{th:M-log-d} are applicable to $\zeta$ and $J_\lambda$ in place of $x$ and $\Sigma$. Hence, repeating the argument from Theorem~\ref{th:covariance-orlicz}, we have that if $n$ satisfies~\eqref{eq:orlicz-ridge-2}, then
\begin{equation*}%\label{eq:q-qhat}
\|\widehat J_\lambda - J_\lambda \| \le 1/2
\end{equation*}
with probability $2/3$, where $\widehat J_\lambda := \Sigma_{\lambda}^{-1/2} \widehat \Sigma \Sigma_{\lambda}^{-1/2}$ (recall that $J_\lambda = \Sigma_{\lambda}^{-1/2} \Sigma \Sigma_{\lambda}$). Equivalently,
\begin{align*}
&&- I/2 \prccq \widehat J_\lambda - J_\lambda \prccq I/2 \quad \\
\Leftrightarrow& &J_\lambda - I/2 \prccq \widehat J_\lambda \prccq J_\lambda + I/2\\
\Leftrightarrow& &\Sigma - \Sigma_\lambda/2 \prccq \widehat \Sigma \prccq \Sigma + \Sigma_\lambda/2\\
\Leftrightarrow& &\frac{1}{2}\Sigma_\lambda \prccq \widehat\Sigma_\lambda \prccq \frac{3}{2}\Sigma_\lambda,
\end{align*}
and we are done.
\end{proof}
